# Supplementary material for: Tracezip: Efficient Distributed Tracing via Trace Compression
Source: arXiv:2502.06318 source file (2025-04-13)
Supplement: Supplementary file 1 [file 09-appendix.tex]

\newpage
\begin{appendices}
\section{Line Charts of Spans Attributes Data}

\begin{figure}[htp]
    \centering
    \includegraphics[width=9cm]{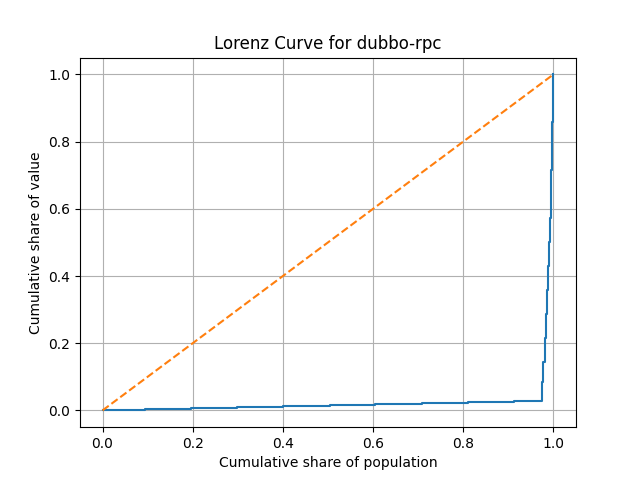}
    \caption{dubbo-rpc lorenz}
\end{figure}

\begin{figure}[htp]
    \centering
    \includegraphics[width=9cm]{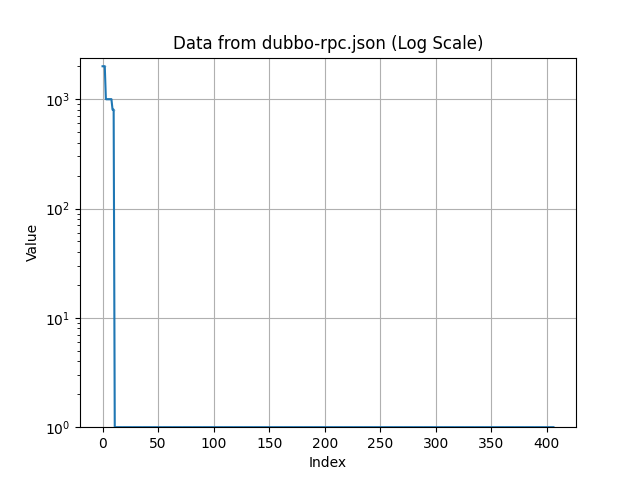}
    \caption{dubbo-rpc}
\end{figure}

\begin{figure}[htp]
    \centering
    \includegraphics[width=9cm]{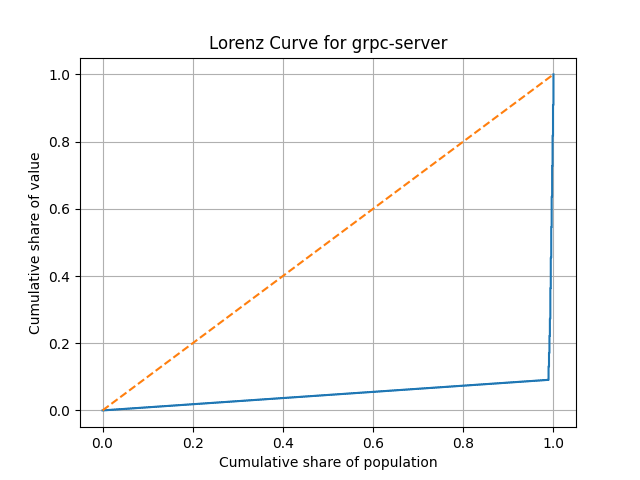}
    \caption{grpc-server lorenz}
\end{figure}

\begin{figure}[htp]
    \centering
    \includegraphics[width=9cm]{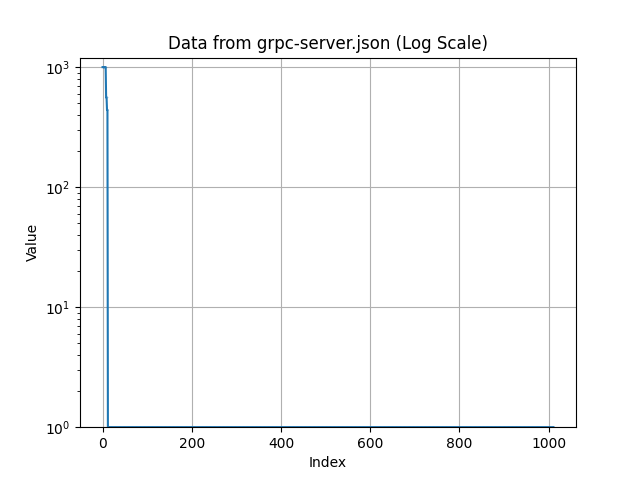}
    \caption{grpc-server}
\end{figure}

\begin{figure}[htp]
    \centering
    \includegraphics[width=9cm]{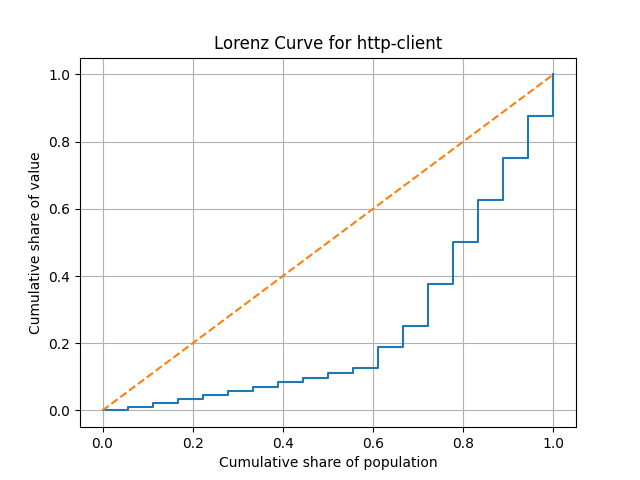}
    \caption{http-client lorenz}
\end{figure}

\begin{figure}[htp]
    \centering
    \includegraphics[width=9cm]{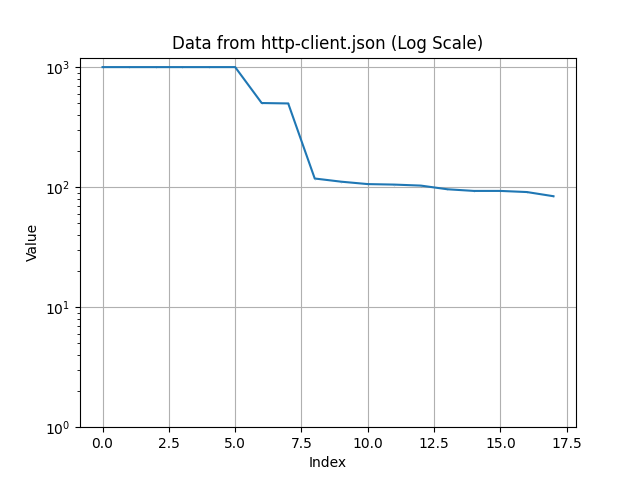}
    \caption{http-client}
\end{figure}

\begin{figure}[htp]
    \centering
    \includegraphics[width=9cm]{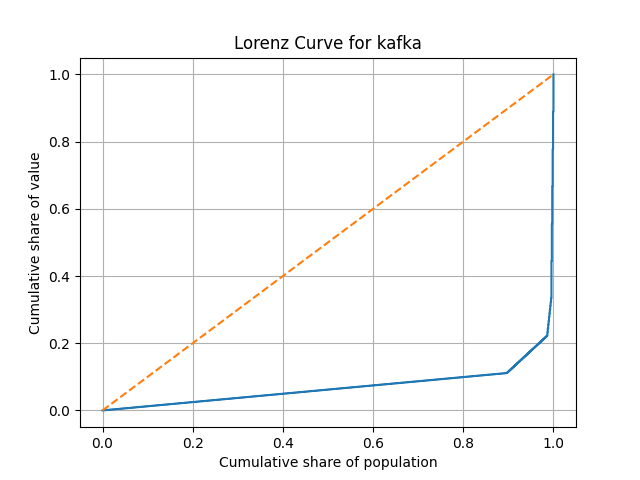}
    \caption{kafka lorenz}
\end{figure}

\begin{figure}[htp]
    \centering
    \includegraphics[width=9cm]{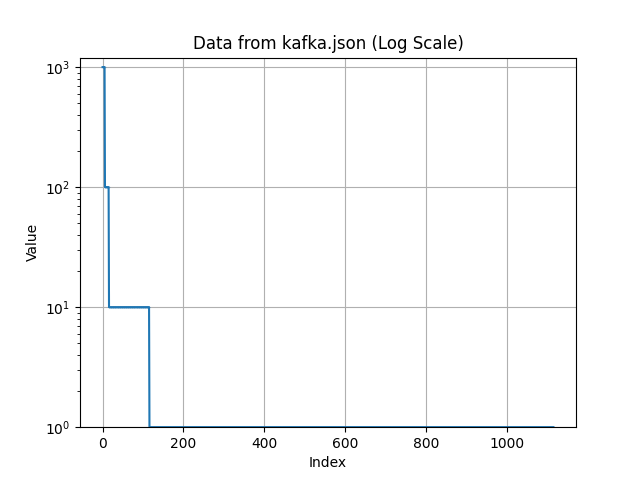}
    \caption{kafka}
\end{figure}

\begin{figure}[htp]
    \centering
    \includegraphics[width=9cm]{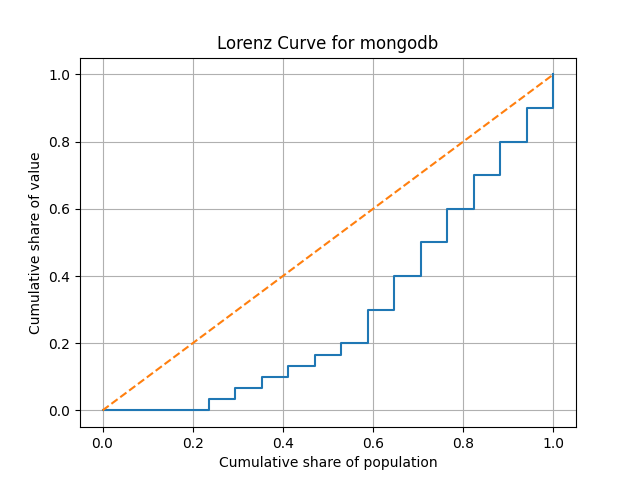}
    \caption{mongodb lorenz}
\end{figure}

\begin{figure}[htp]
    \centering
    \includegraphics[width=9cm]{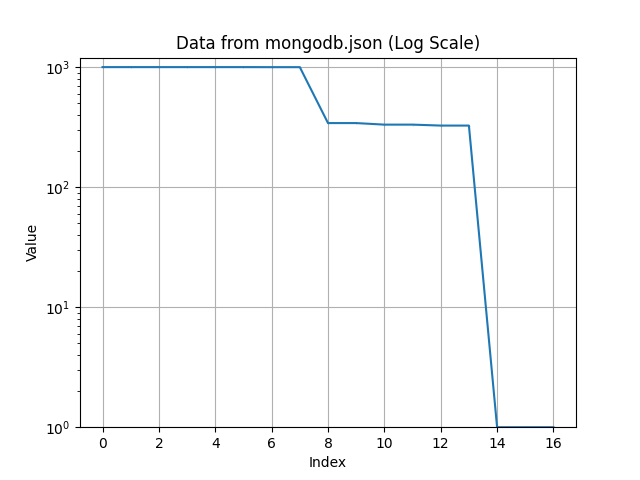}
    \caption{mongodb}
\end{figure}

\begin{figure}[htp]
    \centering
    \includegraphics[width=9cm]{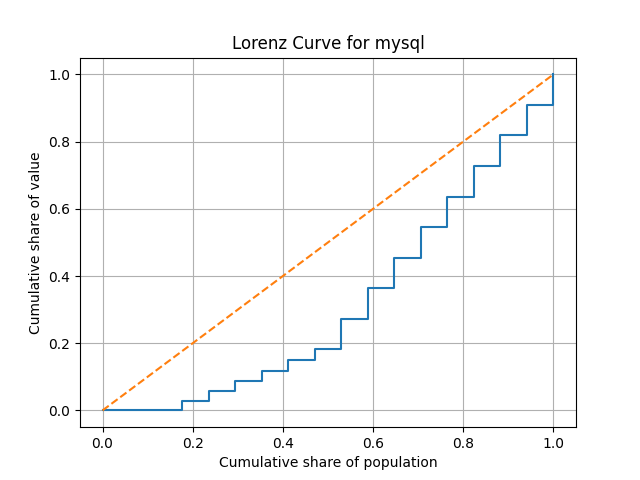}
    \caption{mysql lorenz}
\end{figure}

\begin{figure}[htp]
    \centering
    \includegraphics[width=9cm]{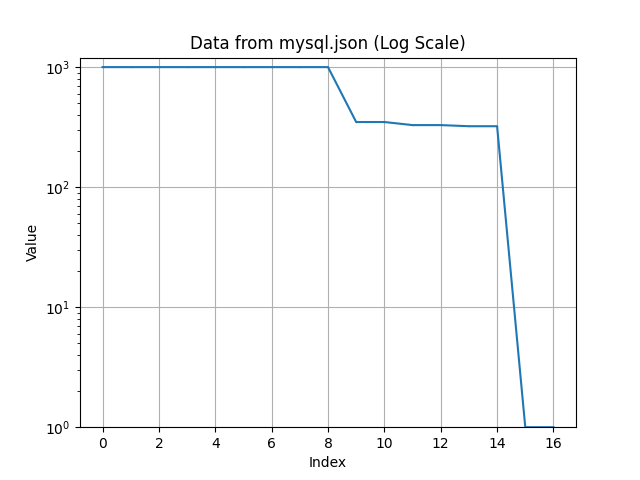}
    \caption{mysql}
\end{figure}

\begin{figure}[htp]
    \centering
    \includegraphics[width=9cm]{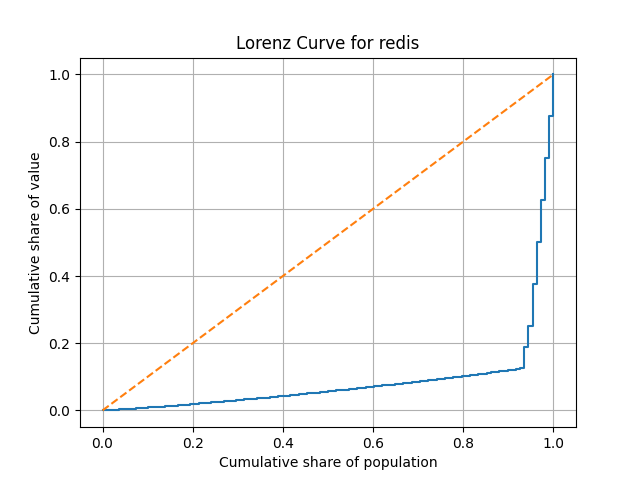}
    \caption{redis lorenz}
\end{figure}

\begin{figure}[htp]
    \centering
    \includegraphics[width=9cm]{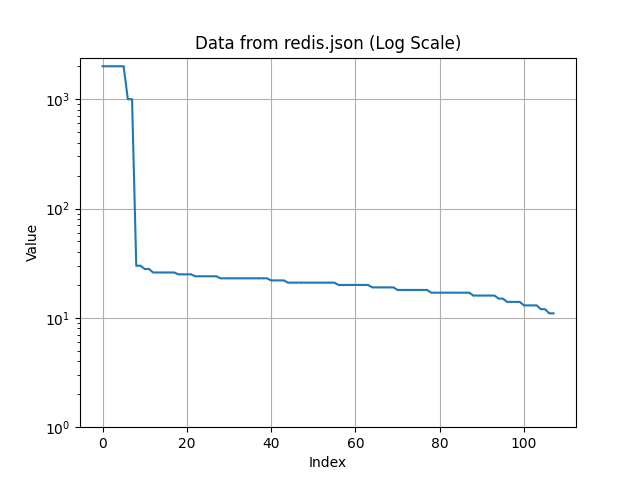}
    \caption{redis}
\end{figure}

\begin{figure}[htp]
    \centering
    \includegraphics[width=9cm]{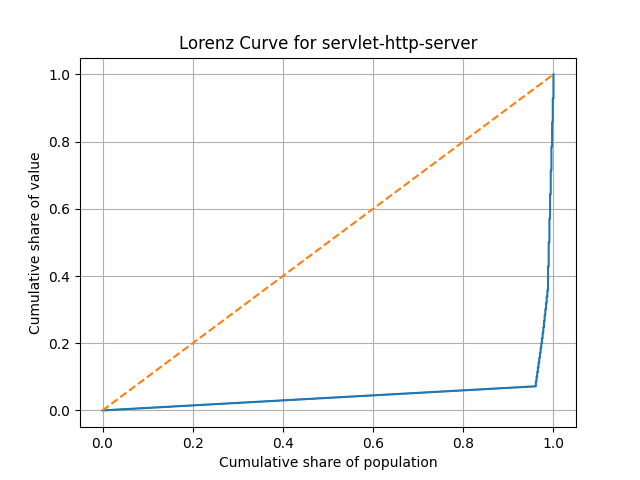}
    \caption{servlet-http-server lorenz}
\end{figure}

\begin{figure}[htp]
    \centering
    \includegraphics[width=9cm]{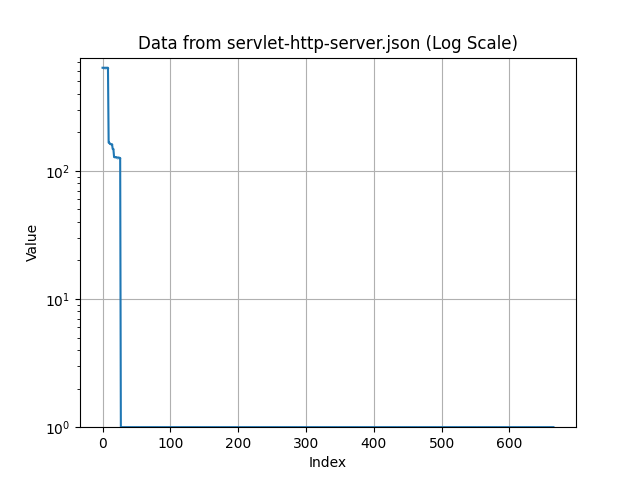}
    \caption{servlet-http-server}
\end{figure}

  \begin{figure}[htp]
    \centering
    \includegraphics[width=9cm]{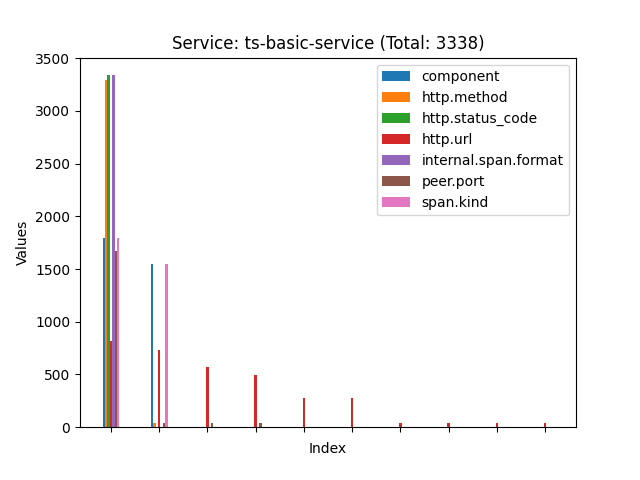}
    \caption{ts-basic-service}
  \end{figure}

  \begin{figure}[htp]
    \centering
    \includegraphics[width=9cm]{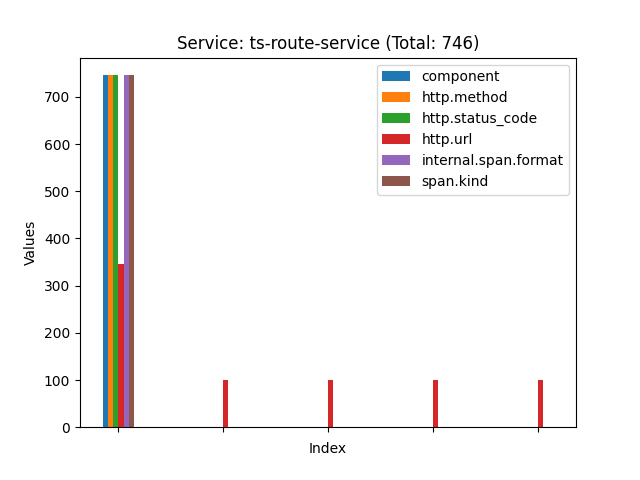}
    \caption{ts-route-service}
  \end{figure}

  \begin{figure}[htp]
    \centering
    \includegraphics[width=9cm]{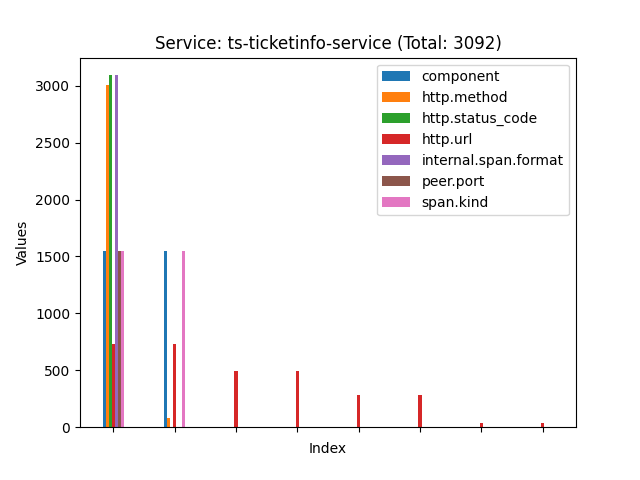}
    \caption{ts-ticketinfo-service}
  \end{figure}

  \begin{figure}[htp]
    \centering
    \includegraphics[width=9cm]{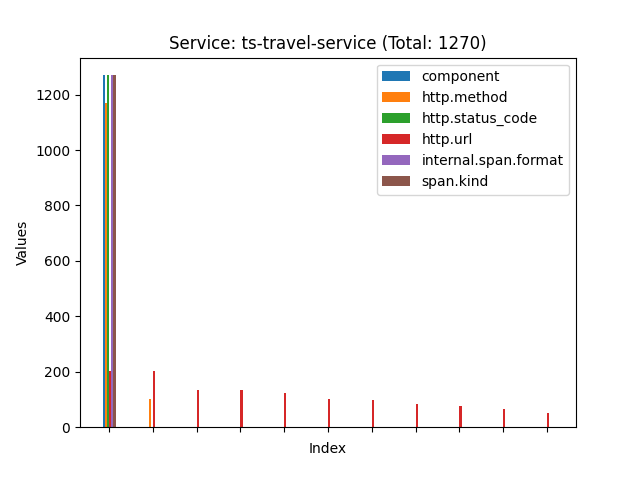}
    \caption{ts-travel-service}
  \end{figure}

  \begin{figure}[htp]
    \centering
    \includegraphics[width=9cm]{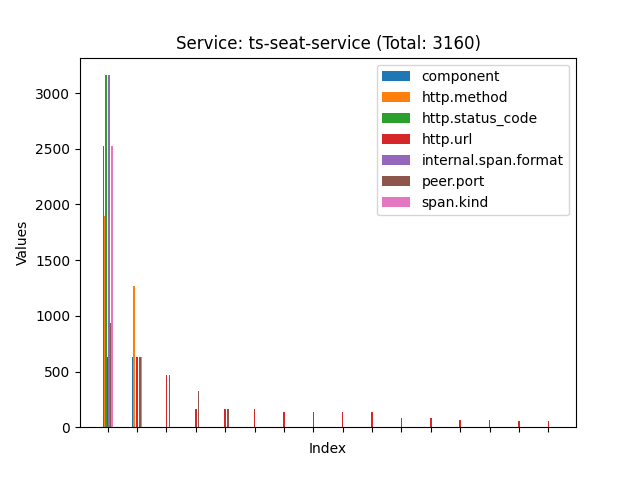}
    \caption{ts-seat-service}
  \end{figure}

  \begin{figure}[htp]
    \centering
    \includegraphics[width=9cm]{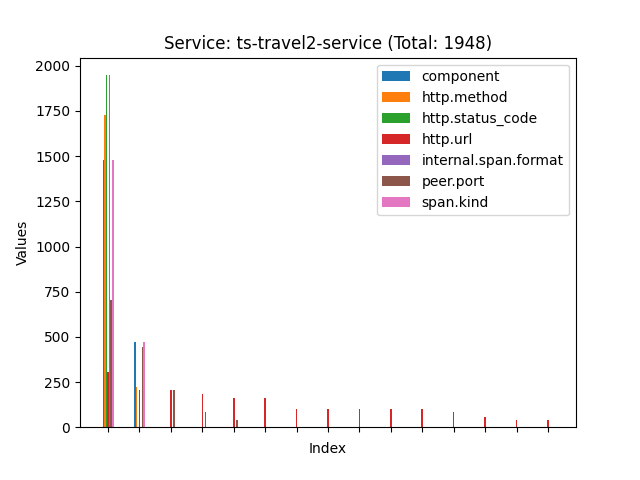}
    \caption{ts-travel2-service}
  \end{figure}

  \begin{figure}[htp]
    \centering
    \includegraphics[width=9cm]{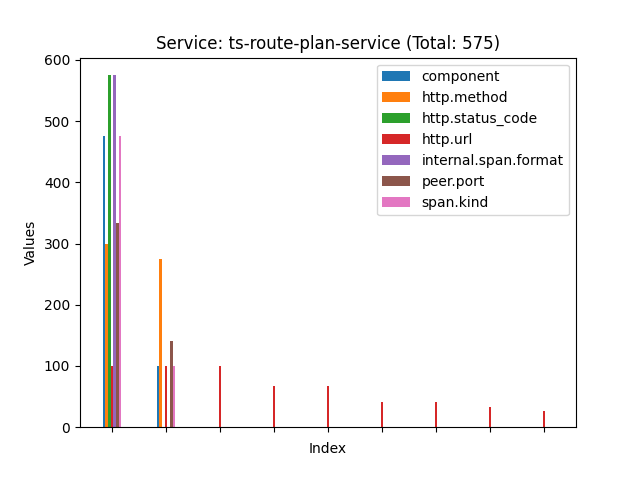}
    \caption{ts-route-plan-service}
  \end{figure}

  \begin{figure}[htp]
    \centering
    \includegraphics[width=9cm]{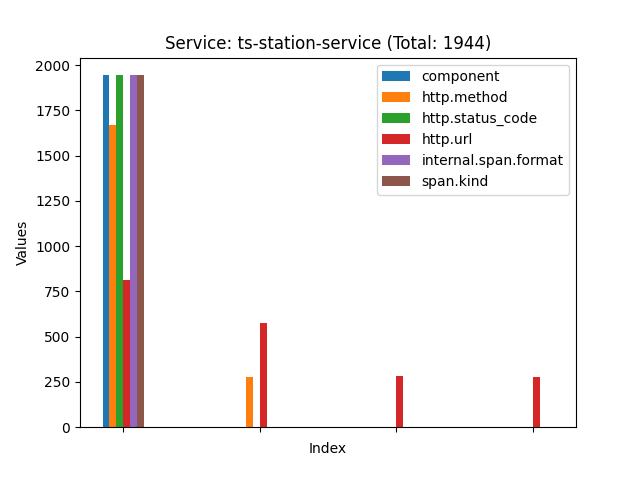}
    \caption{ts-station-service}
  \end{figure}

  \begin{figure}[htp]
    \centering
    \includegraphics[width=9cm]{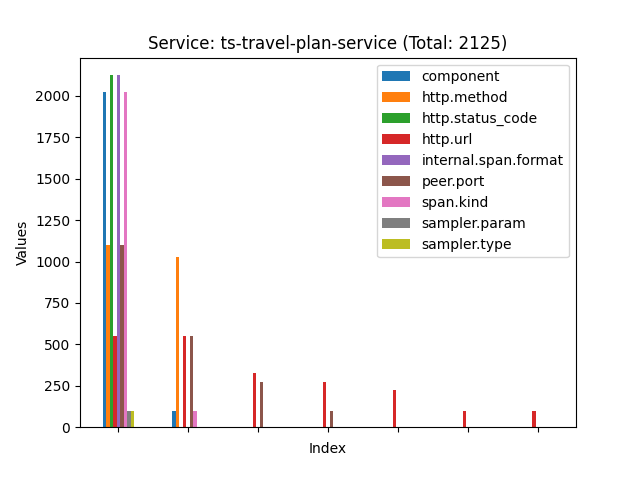}
    \caption{ts-travel-plan-service}
  \end{figure}

\end{appendices}
